# Supplementary material for: Revisiting Embeddings for Graph Neural Networks
Source: arXiv:2209.09338 source file (2022-11-29)
Supplement: Supplementary file 1 [file appendix-models.tex]

\section{Graph Attention Networks}
\label{sec:app:models}

The original paper \textit{Velickovic et al.} \cite{Velickovic:2018we} proposed a new approach to graph representation learning incorporating the popular attention mechanisms of sequence-based tasks.

The basic concept is to provide and attention mechanism $\bm{a}$ which calculates the attention coefficients between a node $v_i$ and its neighbours $\sN_i$, employing self-attention. This attention coefficient between node $v_i$ and a neighbour $v_j$. These coefficients are then normalised to compare across nodes using the \textit{softmax} transform resulting in the final coefficient for a given neighbour $\alpha_{ij}$

\begin{equation}
    \label{eq:GAT}
    \alpha_{ij} = \frac{exp(\mbox{LeakyReLU}(\bm{a}^T[\bm{\theta}\bm{h}_i||\bm{\theta}\bm{h}_j]))}{\sum_{k \in \sN_i} exp(\mbox{LeakyReLU}(\bm{a}^T[\bm{\theta}\bm{h}_i||\bm{\theta}\bm{h}_j]))}
\end{equation}

This attention mechanism occurs for each head in a layer allowing for multi-headed attention. The attention coefficient and weight matrices for each head are denoted with a superscript $k$ where $k \in [K]$ and $K$ is the total number of heads. We can thus relate GAT to the basic MESSAGE-PASSING network equation \ref{eq:messagepassing} as such

\begin{equation}
    \bm{h}^l_i = \mbox{AGGREGATE}_k^K (\sigma(\sum_{j \in \sN_i} \alpha^k_{ij}\bm{\theta}^k \bm{h}^{l-1}_j))
\end{equation}

where AGGREGATE is some aggregation function, the original paper used MEAN and CONCATENATE.

A later paper \textit{Brody et al.} \cite{Brody2021GATv2} questioned the attentiveness of the proposed method and provided the following attention mechanism instead of equation \ref{eq:GAT}

\begin{equation}
    \alpha_{ij} = \frac{exp(\bm{a}^T\mbox{LeakyReLU}(\bm{\theta}[\bm{h}_i||\bm{h}_j]))}{\sum_{k \in \sN_i} exp(\bm{a}^T\mbox{LeakyReLU}(\bm{\theta}[\bm{h}_i||\bm{h}_j]))}
\end{equation}

This graph connection approach allows us to train the attention mechanism $\bm{a}$ across the graph $\mathcal{G}$ without having to train the weight matrix $\bm{\theta}$. So if we are provided with suitable weights we can greatly reduce the training cost. 
